# Supplementary material for: From Birefringent Electrons to a Marginal or Non-Fermi Liquid of Relativistic Spin-1/2 Fermions: An Emergent Superuniversality
Source: arXiv:1802.02134 source file (2018-10-12)
Supplement: Supplementary file 1 [file Supplementary.pdf]

# Supplementary Materials “From Birefringent Electrons to a Marginal or Non-Fermi Liquid of Relativistic Spin-1/2 Fermions: An Emergent Superuniversality”


Bitan Roy,[1] Malcolm P. Kennett,[2] Kun Yang,[3] and Vladimir Juričić[4]

[1] *Max-Planck-Institut für Physik komplexer Systeme, Nöthnitzer Stra. 38, 01187 Dresden, Germany*
[2] *Department of Physics, Simon Fraser University, 8888 University Drive, Burnaby, British Columbia, V5A 1S6, Canada*
[3] *National High Magnetic Field Laboratory and Department of Physics, Florida State University, Tallahassee, Florida 32306, USA*
[4] *Nordita, KTH Royal Institute of Technology and Stockholm University, Roslagstullsbacken 23, 10691 Stockholm, Sweden*


In the present Supplementary Materials we provide the technical details of the following: (a) Computation of the optical conductivity [Sec. I]; (b) Analysis of the effects of long-range Coulomb interaction [Sec. II]; and (c) Analysis of the Gross-Neveu-Yukawa quantum-critical theory [Sec. III] close to a Mott transition, for quasi-relativistic spin-3/2 fermions.

## I. OPTICAL CONDUCTIVITY OF SPIN-3/2 FERMIONS AT $T = 0$

We first present the computation of the optical conductivity of quasi-relativistic spin-3/2 fermions at temperature $T = 0$. The current operator in the $l^{th}$ direction is $j_l = v\left[\Gamma_{l0} + \beta\Gamma_{0l}\right]$, where $\Gamma_{\mu\nu} = \sigma_\mu \otimes \sigma_\nu$ are four-dimensional Hermitian matrices, and $\{\sigma_\mu\}$ represents the set of two-dimensional Pauli matrices, with $\mu = 0, 1, 2, 3$ and $l = 1, \cdots, d$. To find the optical conductivity we first compute the polarization bubble in the presence of external (Matsubara) frequency ($i\Omega$), which in $d$ dimensions is given by

$$\Pi^{(d)}(i\Omega) = \frac{e_0^2}{\hbar\, d} \sum_{l=1}^{d} \Big[ \Pi_{ll}(i\Omega) - \Pi_{ll}(i\Omega = 0) \Big], \tag{1}$$

where $e_0$ is the external electronic test charge,

$$\Pi_{ll}(i\Omega) \;=\; \mathrm{Tr} \int \frac{d^d\mathbf{k}}{(2\pi)^d} \int_{-\infty}^{\infty} \frac{d\omega}{2\pi} \Big[ j_l\, G_{\mathbf{k}}\,(i\omega + i\Omega)\;\, j_l\, G_{\mathbf{k}}\,(i\omega) \Big], \tag{2}$$

and

$$G_{\mathbf{k}}(i\omega) \;=\; \frac{\left[i\omega + H_1(\mathbf{k}) + H_2(\mathbf{k})\right]\; \left[\omega^2 + v^2(1+\beta^2)|\mathbf{k}|^2 - 2H_1(\mathbf{k})H_2(\mathbf{k})\right]}{\left[\omega^2 + v^2(1+\beta)^2|\mathbf{k}|^2\right]\left[\omega^2 + v^2(1-\beta)^2|\mathbf{k}|^2\right]}, \tag{3}$$

is the fermionic Green's function in terms of Matsubara frequency $i\omega$, and

$$H_1(\mathbf{k}) = v \sum_{j=1}^{d} \Gamma_{j0} k_j, \quad H_2(\mathbf{k}) = v\beta \sum_{j=1}^{d} \Gamma_{0j} k_j, \tag{4}$$

with

$$H_{\frac{3}{2}}(\mathbf{k}) = H_1(\mathbf{k}) + H_2(\mathbf{k}).$$

After completing the trace algebra we arrive at the following compact expression for $\Pi^{(d)}(i\Omega)$

$$\Pi^{(d)}(i\Omega) = \frac{e_0^2 N_f}{d\hbar} \int \frac{d^d\mathbf{k}}{(2\pi)^2} \int_{-\infty}^{\infty} \frac{d\omega}{2\pi} \left[ \frac{N(i\Omega, i\omega, k)}{D(i\Omega, i\omega, k)} - \frac{N(0, i\omega, k)}{D(0, i\omega, k)} \right], \tag{5}$$

where

$$\begin{aligned} N(i\Omega, i\omega, k) \;&=\; 8\omega(\omega+\Omega)\left[k^4(1+\beta^2)(1-\beta^2)^2 + (1+\beta^2)\omega^2(\omega+\Omega)^2 \right. \\ &+\; \left. k^2\left\{2(1-\beta^2)^2\omega^2 + 2(1-\beta^2)\omega\Omega + (1+\beta^4)\Omega^2\right\}\right], \\ D(i\Omega, i\omega, k) \;&=\; \left[\omega^2 + (1+\beta)^2k^2\right]\left[\omega^2 + (1-\beta)^2k^2\right]\left[(\omega+\Omega)^2 + (1+\beta)^2k^2\right]\left[(\omega+\Omega)^2 + (1-\beta)^2k^2\right]. \end{aligned} \tag{6}$$

Performing the frequency integral using the residue technique we find

$$\Pi^{(d)}(i\Omega) = \frac{2e_0^2 N_f}{\hbar\, d} \int \frac{d^d\mathbf{k}}{(2\pi)^2} \left[\frac{4k}{4k^2+\Omega^2} - \frac{1}{k}\right] = \frac{2e_0^2 N_f \Omega^{d-1}}{\hbar\, d} \frac{S_d}{(2\pi)^d} \left[2^{-d}\, \pi \sec\left(\frac{\pi d}{2}\right)\right], \tag{7}$$

where $S_d$ is the surface area of a $d$-dimensional unit sphere, which leads to

$$\Pi^{(2)}(i\Omega) = -\frac{N_f e_0^2}{2\pi\hbar}\frac{\Omega\pi}{4}, \quad \Pi^{(3)}(i\Omega) = \frac{N_f e_0^2}{12\pi^2\hbar}\frac{\Omega^2}{v\epsilon}, \tag{8}$$

where $\epsilon = 3-d$. Physically, $1/\epsilon \equiv \ln(2v\Lambda_0/\Omega)$ captures the screening of external charge in the medium by gapless fermions. Performing analytic continuation to real frequency according to $i\Omega \to \omega + i\delta$ and using the Kubo formula

$$\sigma_{ll}^{(d)}(\omega) = \lim_{\delta\to 0} \frac{\Im\Pi_{ll}(i\Omega \to \omega + i\delta)}{\omega}, \tag{9}$$

we find the optical conductivity in a relativistic spin-3/2 system to be

$$\sigma_{ll}^{(2)}(\omega) = \frac{e_0^2}{h}\frac{\pi N_f}{4}, \quad \sigma_{ll}^{(3)}(\omega) = \frac{e_0^2}{h}\frac{N_f\omega}{6v}, \tag{10}$$

respectively in $d=2$ and $d=3$.

## II. LONG-RANGE COULOMB INTERACTION

Next we present the details of the field theory analysis regarding the effects of the long-range Coulomb interaction on a collection of relativistic spin-3/2 fermions. The imaginary-time ($\tau$) action capturing the instantaneous Coulomb interaction is given by

$$S_C = \int d\tau d^d\mathbf{r}\; d^d\mathbf{r}' \rho(\tau,\mathbf{r}) V(\mathbf{r}-\mathbf{r}')\rho(\tau,\mathbf{r}'), \tag{11}$$

where $V(\mathbf{r}-\mathbf{r}') = e^2/|\mathbf{r}-\mathbf{r}'|$ and $\rho(\tau,\mathbf{r}) = \Psi^\dagger(\tau,\mathbf{r})\Psi(\tau,\mathbf{r})$ is the fermionic density. In reciprocal space the Coulomb interaction $V(\mathbf{k}) \sim e^2/|\mathbf{k}|^{d-1}$ is an analytic (a non-analytic) function of momentum respectively in three (two) dimensions. The correction to the fermionic self-energy due to the long-range Coulomb interaction is

$$\Sigma(i\Omega,\mathbf{q}) = (ie)^2 \int \frac{d^D\mathbf{k}}{(2\pi)^D} \int_{-\infty}^{\infty} \frac{d\omega}{2\pi} \frac{G(i\omega,\mathbf{k})}{|\mathbf{k}-\mathbf{q}|^{d-1}} = -\frac{e^2}{2v} \int \frac{d^D\mathbf{k}}{(2\pi)^D} \frac{H_1(\mathbf{k})}{|\mathbf{k}|\;|\mathbf{k}-\mathbf{q}|^{d-1}}, \tag{12}$$

after we complete the integral over the Matsubara frequency ($\omega$), where $D = d-\epsilon$. In this method the ultraviolet divergence of the self-energy correction appears as $1/\epsilon$. Now we perform the integral over momentum by introducing a Feynman parameter ($x$), yielding

$$\Sigma(i\Omega,\mathbf{q}) = -\frac{e^2}{2v}\left[\frac{\Gamma[d/2]}{\Gamma[1/2]\Gamma[(d-1)/2]} \int_0^1 dx\, x^{\frac{d-3}{2}} (1-x)^{-1/2} \int \frac{d^D\mathbf{k}}{(2\pi)^D} \frac{H_1(\mathbf{k})}{\left[(\mathbf{k}-x\mathbf{q})^2 + x(1-x)q^2\right]^{d/2}}\right]. \tag{13}$$

After making the shift in the momentum variable according to $\mathbf{k} - x\mathbf{q} \to \mathbf{k}$, we obtain

$$\begin{aligned}\Sigma(i\Omega,\mathbf{q}) &= -H_1(\mathbf{q})\frac{e^2}{2v}\left[\frac{\Gamma[d/2]}{\Gamma[1/2]\Gamma[(d-1)/2]} \int_0^1 dx\, x^{\frac{d-3}{2}}(1-x)^{-1/2} \int \frac{d^D\mathbf{k}}{(2\pi)^D} \frac{1}{[k^2 + x(1-x)q^2]^{d/2}}\right] \\ &= -H_1(\mathbf{q})\frac{e^2}{2v}\frac{\Gamma[\epsilon/2]\, q^{-\epsilon}}{\Gamma[1/2]\Gamma[(d-1)/2]} \int_0^1 dx\, x^{\frac{d-1-\epsilon}{2}} (1-x)^{-\frac{1+\epsilon}{2}}. \end{aligned} \tag{14}$$

Now, specifically for two ($d=2$) and three ($d=3$) dimensions we obtain

$$\Sigma(i\Omega,\mathbf{q}) = -\alpha\, H_1(\mathbf{q})\, \frac{q^{-\epsilon}}{\epsilon} \begin{cases} (8\pi)^{-1} & \text{for } d=2 \\ (6\pi^2)^{-1} & \text{for } d=3 \end{cases}$$

In three dimensions ($d = 3$) we also need to account for the renormalization of charge since the Coulomb interaction $V(\mathbf{k}) \sim e^2/|\mathbf{k}|^2$ is an *analytic* function of momentum. The polarization bubble in $d = 3$ reads as

$$\Pi_{00}(i\Omega, \mathbf{q}) = -(ie)^2 \int \frac{d^D\mathbf{k}}{(2\pi)^D} \int_{-\infty}^{\infty} \frac{d\omega}{2\pi} \, \mathbf{Tr} \, \left[ G_{\mathbf{k}}(i\omega) \, G_{\mathbf{k}+\mathbf{q}}(i\Omega + i\omega) \right]. \tag{15}$$

The analytical expression for $\Pi_{00}(i\Omega, \mathbf{q})$ is extremely lengthy and not instructive, hence we use mathematica to obtain the final expression

$$\Pi_{00}(i\Omega, \mathbf{q}) = -\frac{N_f e^2}{6v\pi^2} \, q^2 \, \frac{q^{-\epsilon}}{\epsilon}. \tag{16}$$

Notice that the final expression is independent of the birefringence parameter $\beta$: this polarization bubble is the same one from which we obtained optical conductivity, but here computed at both a finite frequency and momentum.

From the computation of the self-energy for fermionic and bosonic fields we finally arrive at the following renormalization group flow equations

$$\frac{dv}{d\ell} = \frac{\alpha v}{C_d} \equiv \frac{e^2}{C_d}, \quad \frac{d\beta}{d\ell} = -\frac{\alpha\beta}{C_d}, \quad \frac{d\alpha}{d\ell} = -(1 + N_f \delta_{d,3}) \frac{\alpha^2}{C_d}, \tag{17}$$

where $\alpha = e^2/v$ is the fine structure constant, $\ell \equiv \ln(\Lambda_0/\Lambda) > 1$ is the logarithm of the running renormalization group scale, $C_2 = 8\pi$ and $C_3 = 6\pi^2$. The physical implications of this set of coupled RG flow equations are discussed in the main text of the paper and also displayed in Fig. 1 of main paper.

## III. GROSS-NEVEU YUKAWA THEORY

Finally, we present the details of the analysis for effective Gross-Neveu-Yukawa (GNY) theory when the system resides in close proximity to a Mott transition. We focus here only on the orderings $\langle \Psi^\dagger M_\alpha \Psi \rangle \neq 0$ that yield fully and isotropically gapped Fermi points. Such a situation can be realized when $\left\{ M_\alpha, \tilde{\eta} \otimes H_{\frac{3}{2}}(\mathbf{k}) \right\} = 0$, where

$$H_{\frac{3}{2}}(\mathbf{k}) = v \sum_{j=1}^{d} \left[ \Gamma_{j0} k_j + \beta \Gamma_{0j} k_j \right], \tag{18}$$

in dimensions $d = 2$ and 3. Specifically for $d = 2$, $\tilde{\eta} \equiv \eta_0$ is a two-dimensional identity matrix, and the Hamiltonian is obtained from the spin-independent hopping of fermions on a generalized $\pi$-flux square lattice in the low-energy limit [1]. For such a system the set of Pauli matrices $\{\eta_\mu\}$ operate on the spin index. In $d = 3$, $\tilde{\eta} \equiv \eta_3$, the Hamiltonian describes a strong spin-orbit coupled system, and $\{\eta_\mu\}$ operate on the valley index.

Indpendent of the detailed origin of the order parameter, the effective Euclidean action describing such a quantum phase transition is given by $S = \int d^D x d\tau \mathcal{L}$, where the Lagrangian $\mathcal{L} = \mathcal{L}_f + \mathcal{L}_Y + \mathcal{L}_b$, with

$$\mathcal{L}_f = \Psi^\dagger \left[ \partial_\tau + \tilde{\eta} \otimes H_{\frac{3}{2}}(\mathbf{k} \to -i\nabla) \right] \Psi, \quad \mathcal{L}_Y = g \sum_{\alpha=1}^{N_b} \Phi_\alpha \Psi^\dagger M_\alpha \Psi,$$
$$L_b = \sum_{\alpha=1}^{N_b} \left[ -\frac{1}{2} \Phi_\alpha \left( \partial_\tau^2 + v_B^2 \sum_{j=1}^{d} \partial_\mu^2 - m_b^2 \right) \Phi_\alpha + \frac{\lambda}{4!} [\Phi_\alpha^2]^2 \right], \tag{19}$$

and $N_b$ counts the number of real order-parameter components. Since both Yukawa ($g$) and four-boson ($\lambda$) couplings are marginal in $d = 3$, we can perform a controlled perturbative RG calculation about three dimensions in terms of a small parameter $\epsilon = 3 - d$ [2]. Next we present fermionic and bosonic self-energy corrections.

### A. Fermionic self-energy

The fermionic self-energy correction is given by

$$\Sigma(i\nu, \mathbf{k}) = g^2 \sum_{\alpha=1}^{N_b} \int \frac{d^d\mathbf{p}}{(2\pi)^d} \int_{-\infty}^{\infty} \frac{d\omega}{2\pi} \, M_\alpha \, G_{\mathbf{p}}(i\omega) \, M_\alpha \, G^{\mathrm{B}}_{\mathbf{k}-\mathbf{p}}(i\nu - i\omega), \tag{20}$$

where $G^{\mathrm{B}}_{\mathbf{k}}(i\omega) = \left[\omega^2 + v_B^2 k^2 + m^2\right]^{-1}$ is the bosonic Green's function. Since we perform the calculation about the upper critical dimension $d = 3$, where propagators are analytic functions of external momentum and frequency, we enjoy the liberty of computing the self-energy diagram for (i) zero external momentum, yielding $\Sigma(i\nu, 0)$, and (ii) zero external frequency, yielding $\Sigma(0, \mathbf{k})$, finally leading to $\Sigma(i\nu, \mathbf{k}) = \Sigma(i\nu, 0) + \Sigma(0, \mathbf{k})$.

The self-energy for zero external momentum $\Sigma(i\nu, 0)$ takes the form

$$\begin{aligned}
\Sigma(i\nu, 0) &= g^2 N_b \int \frac{d^d\mathbf{p}}{(2\pi)^d} \int_{-\infty}^{\infty} \frac{d\omega}{2\pi} \frac{i\omega\left[\omega^2 + v^2(1+\beta^2)\mathbf{p}^2 - 2H_1(\mathbf{p})H_2(\mathbf{p})\right]}{\left[\omega^2 + v^2(1+\beta)^2|\mathbf{p}|^2\right]\left[\omega^2 + v^2(1-\beta)^2|\mathbf{p}|^2\right]\left[(\omega-\nu)^2 + v_B^2|\mathbf{p}|^2\right]} \\
&= (i\nu)\,\frac{N_b g^2}{2}\left[\sum_{\tau=\pm} J_\tau + \hat{M}\sum_{\tau=\pm}\tau J_\tau\right],
\end{aligned} \tag{21}$$

after completing the frequency integral (using the residue technique), with $\hat{M} = i\sum_{j=1}^{d}\Gamma_{j0}\Gamma_{0j}$ and

$$J_\tau = \int \frac{d^d\mathbf{p}}{(2\pi)^d} \frac{1}{2v_B|\mathbf{p}|\left[p^2\left(v(1+\tau\beta)+v_B\right)^2 + \nu^2\right]} = \frac{\nu^{-\epsilon}}{4\pi^2 v_B} \frac{1}{\left[v(1+\tau\beta)+v_B\right]^2}\,\frac{1}{\epsilon} + \mathcal{O}(1). \tag{22}$$

Therefore, we finally obtain

$$\Sigma(i\nu, 0) = (i\nu)\frac{N_b\, g^2}{4\pi^2 v_B\left[(v+v_B)^2 - \beta^2 v^2\right]^2}\left[(v+v_B)^2 + v^2\beta^2 - 2\beta\hat{M}\, v(v+v_B)\right]\frac{\nu^{-\epsilon}}{\epsilon} + \mathcal{O}(1). \tag{23}$$

The renormalized coefficient of $\hat{M}$ is kept pinned to *zero* and we can neglect the generation of new terms proportional to $\hat{M}$. The renomalization condition $i\nu Z_\Psi + \Sigma(i\nu, 0) = i\nu$, yields the fermionic wave-function renormalization

$$Z_\Psi = 1 - N_b \frac{g^2 k^{-\epsilon}}{4\pi^2\epsilon}\,\frac{(v+v_B)^2 + \beta^2 v^2}{v_B\left[(v+v_B)^2 - v^2\beta^2\right]^2}. \tag{24}$$

Now we proceed with the computation of self-energy for zero external frequency, given by

$$\begin{aligned}
\Sigma(0, \mathbf{k}) &= N_b\, g^2 \int \frac{d^d\mathbf{p}}{(2\pi)^d}\int_{-\infty}^{\infty}\frac{d\omega}{2\pi}\frac{\left[i\omega - H_1(\mathbf{p} - H_2(\mathbf{p})\right]\left[\omega^2 + v^2(1+\beta)^2|\mathbf{p}|^2 - 2H_1(\mathbf{p})H_2(\mathbf{p})\right]}{\left[\omega^2 + v^2(1+\beta)^2|\mathbf{p}|^2\right]\left[\omega^2 + v^2(1-\beta)^2|\mathbf{p}|^2\right]\left[\omega^2 + v_B^2(\mathbf{k}-\mathbf{p})^2\right]} \\
&= -\frac{N_b\, g^2}{4vv_B}\sum_{\tau=\pm}\int\frac{d^d\mathbf{p}}{(2\pi)^d}\frac{H_1(\mathbf{p}) + \frac{\tau}{\beta}H_2(\mathbf{p})}{|\mathbf{p}||\mathbf{k}-\mathbf{p}|\left[v(1+\tau\beta)|\mathbf{p}| + v_B|\mathbf{k}-\mathbf{p}|\right]} = -\frac{N_b\, g^2}{4vv_B}\left[I_1(\mathbf{k}) + I_2(\mathbf{k})\right],
\end{aligned} \tag{25}$$

after completing the integral over Matsubara frequency ($\omega$). The two integral expressions in the last equation read as

$$\begin{aligned}
I_1(\mathbf{k}) &= \sum_{\tau=\pm}\int\frac{d^d\mathbf{p}}{(2\pi)^d}\frac{v(1+\tau\beta)\left(H_1(\mathbf{p}+\mathbf{k}) + \frac{\tau}{\beta}H_2(\mathbf{p}+\mathbf{k})\right)}{|\mathbf{p}|\left[v^2(1+\tau\beta)^2|\mathbf{p}+\mathbf{k}|^2 - v_B^2 p^2\right]} \\
&= \sum_{\tau=\pm}\frac{v(1+\tau\beta)\left[2v^2(1+\tau\beta)^2 - 6v_B^2\right]}{3\left[v^2(1+\tau\beta)^2 - v_B^2\right]^2}\left[H_1(\mathbf{k}) + \frac{\tau}{\beta}H_2(\mathbf{k})\right]\frac{k^{-\epsilon}}{4\pi^2\epsilon} + \mathcal{O}(1),
\end{aligned} \tag{26}$$

$$I_2(\mathbf{k}) = -\sum_{\tau=\pm}\int\frac{d^d\mathbf{p}}{(2\pi)^d}\frac{v_B\left(H_1(\mathbf{p}) + \frac{\tau}{\beta}H_2(\mathbf{p})\right)}{|\mathbf{p}|\left[v^2(1+\tau\beta)^2|\mathbf{p}|^2 - v_B^2|\mathbf{k}-\mathbf{p}|^2\right]}$$

$$= \sum_{\tau=\pm} \frac{4v_B^3 v}{3\left[v^2(1+\tau\beta)^2 - v_B^2\right]^2} \left[H_1(\mathbf{k}) + \frac{\tau}{\beta} H_2(\mathbf{k})\right] \frac{k^{-\epsilon}}{4\pi^2\epsilon} + \mathcal{O}(1). \tag{27}$$

We then arrive at the final expression

$$\Sigma(0,\mathbf{k}) = N_b \frac{g^2 k^{-\epsilon}}{4\pi^2\epsilon} \left[ -\frac{(v+v_B)^2(v+2v_B) - v^3\beta^2}{3vv_B\left[(v+v_B)^2 - v^2\beta^2\right]^2} H_1(\mathbf{k}) + \frac{4vv_B + 3v_B^2 - v^2(\beta^2-1)}{3v_B\left[(v+v_B)^2 - v^2\beta^2\right]^2} H_2(\mathbf{k}) \right]. \tag{28}$$

The renormalization condition ($Z_v$) for the mean Fermi velocity ($v$) reads as

$$Z_\Psi Z_v + N_b \frac{g^2 k^{-\epsilon}}{4\pi^2\epsilon} \frac{(v+v_B)^2(v+2v_B) - v^3\beta^2}{3vv_B\left[(v+v_B)^2 - v^2\beta^2\right]^2} = 1 \Rightarrow Z_v = 1 + \frac{g^2 k^{-\epsilon}}{4\pi^2\epsilon} A(v, v_B, \beta), \tag{29}$$

where

$$A(v, v_B, \beta) = N_b \left[ \frac{(v+v_B)^2 + \beta^2 v^2}{v_B\left[(v+v_B)^2 - v^2\beta^2\right]^2} - \frac{(v+v_B)^2(v+2v_B) - v^3\beta^2}{3vv_B\left[(v+v_B)^2 - v^2\beta^2\right]^2} \right] = N_b \frac{2(v-v_B)(v+v_B)^2 + 4v^3\beta^2}{3vv_B\left[(v+v_B)^2 - v^2\beta^2\right]}. \tag{30}$$

The renormalization condition ($Z_\beta$) for the birefringent parameter ($\beta$) is given by

$$Z_\Psi Z_v Z_\beta - N_b \frac{g^2 k^{-\epsilon}}{4\pi^2\epsilon} \frac{4vv_B + 3v_B^2 + v^2(1-\beta^2)}{3v_B\left[v(1+\beta) + v_B\right]^2\left[v(1-\beta)+v_B\right]^2} = 1 \Rightarrow Z_\beta = 1 + \frac{g^2 k^{-\epsilon}}{4\pi^2\epsilon} S(v, v_B, \beta), \tag{31}$$

where

$$S(v, v_B, \beta) = N_b \left[ \frac{4vv_B + 3v_B^2 + v^2(1-\beta^2)}{3v_B\left[(v+v_B)^2 - v^2\beta^2\right]^2} + \frac{(v+v_B)^2(v+2v_B) - v^3\beta^2}{3vv_B\left[(v+v_B)^2 - v^2\beta^2\right]^2} \right] = 2N_b \frac{4vv_B(v+v_B) + v_B^3 + v^3(1-\beta^2)}{3vv_B\left[(v+v_B)^2 - v^2\beta^2\right]}. \tag{32}$$

From the above conditions we immediately arrive at the RG flow equations for $v$ and $\beta$, respectively given by

$$\frac{dv}{d\ell} = -v\frac{g^2}{4\pi^2} A(v, v_B, \beta), \quad \frac{d\beta}{d\ell} = -\beta \frac{g^2}{4\pi^2} S(v, v_B, \beta). \tag{33}$$

Also note that the flow of the parameter $\beta v$, given by

$$\frac{d(\beta v)}{d\ell} = -(\beta v)\frac{g^2}{4\pi^2}\left[A(v, v_B, \beta) + S(v, v_B, \beta)\right] \equiv -N_b(\beta v)\frac{g^2}{2\pi^2} \left[ \frac{vv_B(v+v_B)\left(4 + \frac{v}{v_B} - \frac{v_B}{v}\right) + v^3(1+\beta^2) + v_B^3}{3vv_B\left[(v+v_B)^2 - v^2\beta^2\right]} \right] \tag{34}$$

suggests that $\beta v$ is always an irrelevant parameter, irrespective of weather $v > v_B$ or $v_B > v$ in the bare theory. Now we proceed with the computation of bosonic self-energy correction.

### B. Bosonic self-energy

The formal expression for the bosonic self-energy diagram due to Yukawa coupling reads as

$$\Pi_B(\nu, \mathbf{k}) = -\frac{g^2}{2}\mathrm{Tr}\left[ \int \frac{d^d\mathbf{p}}{(2\pi)^d} \int_{-\infty}^{\infty} \frac{d\omega}{2\pi} M_\alpha G_{\mathbf{p}}(i\omega) M_\alpha G_{\mathbf{k}+\mathbf{p}}(i\omega + i\nu) \right]. \tag{35}$$

We compute this expression for (a) zero external momentum and (b) zero external frequency. For $\mathbf{k} = 0$ we obtain

$$\Pi_B(\nu, 0) = -N_f \frac{g^2}{2v^d} \int \frac{d^d\mathbf{p}}{(2\pi)^d} \frac{-8|\mathbf{p}|\left[4p^2(1-\beta^2) + \nu^2\right]}{16p^4(1-\beta^2)^2 + 8p^2\nu^2(1+\beta^2) + \nu^4} = -N_f\nu^2 \left[\frac{g^2}{8\pi^2 v^3} \frac{\nu^{-\epsilon}}{\epsilon}\right] \frac{1+3\beta^2}{(1-\beta^2)^3} + \mathcal{O}(1), \tag{36}$$

which immediately yields the bosonic field renormalization condition

$$Z_\Phi = 1 - \frac{g^2 N_f}{8\pi^2 v^3} \frac{1+3\beta^2}{(1-\beta^2)^3} \frac{\nu^{-\epsilon}}{\epsilon} + \mathcal{O}(1). \tag{37}$$

Next we compute the bosonic self-energy for zero external frequency, yielding

$$\Pi_B(0,\mathbf{k}) = \frac{g^2 N_f}{v^d(1-\beta^2)} \int \frac{d^d\mathbf{p}}{(2\pi)^d} \frac{\left[|\mathbf{p}||\mathbf{k}+\mathbf{p}| + p^2 + \mathbf{k}\cdot\mathbf{p}\right]\left[\left(|\mathbf{k}+\mathbf{p}|+|\mathbf{p}|\right)^2 - \beta^2 k^2\right]}{|\mathbf{p}||\mathbf{k}+\mathbf{p}|\left(|\mathbf{k}+\mathbf{p}|+|\mathbf{p}|\right)\left[(1+\beta)|\mathbf{k}+\mathbf{p}|+(1-\beta)|\mathbf{p}|\right]\left[(1-\beta)|\mathbf{k}+\mathbf{p}|+(1+\beta)|\mathbf{p}|\right]}$$
$$= -\left[\frac{g^2 N_f}{8\pi^2 v^3}\,\frac{3+2\beta^2}{3(1-\beta^2)}\right](v^2k^2)\frac{k^{-\epsilon}}{\epsilon} + \mathcal{O}(1). \tag{38}$$

The renormalization group condition for the bosonic velocity $(v_B)$ reads as

$$Z_\Phi Z_{v_B}^2 + \left[\frac{g^2 N_f}{8\pi^2 v^3}\,\frac{3+2\beta^2}{3(1-\beta^2)}\right]\frac{k^{-\epsilon}}{\epsilon}\,\frac{v^2}{v_B^2} = 1 \Rightarrow Z_{v_B} = 1 + \frac{g^2 N_f k^{-\epsilon}}{16\pi^2 v^3 \epsilon}\left[\frac{1+3\beta^2}{(1-\beta^2)^2} - \frac{v^2}{v_B^2}\left(1+\frac{2\beta^2}{3}\right)\right]\frac{1}{1-\beta^2}. \tag{39}$$

From $Z_{v_B}$ we immediately obtain the following RG flow equation for the bosonic velocity $v_B$

$$\frac{dv_B}{d\ell} = -\frac{g^2}{8\pi^2}\frac{N_f v_B}{2v^3(1-\beta^2)}\left[\frac{1}{1-\beta^2} - \frac{v^2}{v_B^2} + \beta^2\left\{\frac{4}{(1-\beta^2)^2} - \frac{2v^2}{3v_B^2}\right\}\right]. \tag{40}$$

The analysis of above coupled flow equations is discussed in the main text of the paper.

---


[1] M. P. Kennett, N. Komeilizadeh, K. Kaveh, and P. M. Smith, Phys. Rev. A **83**, 053636 (2011).
[2] J. Zinn-Justin, *Quantum Field Theory and Critical Phenomena* (Oxford University Press, Oxford, UK, 2002).
